# Supplementary material for: Diffusion idea exploration for art generation
Source: arXiv:2307.04978 source file (2023-07-11)
Supplement: Supplementary file 1 [file appendix.tex]

\appendix
\chapter{Appendix}
\label{appendix} 

\section{Qualitative Results}

More qualitative result images of both CoDraw and iCLEVR datasets.

\begin{figure}[htb!]
  \centering
   \centerline{\includegraphics[width=1\linewidth]{figures/codraw_2.png}}
   \caption{CoDraw manipulation sequence results}
   \label{fig:seq2codraw}
\end{figure}

\begin{figure}[htb!]
  \centering
   \centerline{\includegraphics[width=1\linewidth]{figures/codraw_3.png}}
   \caption{CoDraw manipulation sequence results}
   \label{fig:seq3codraw}
\end{figure}

\begin{figure}[htb!]
  \centering
   \centerline{\includegraphics[width=1\linewidth]{figures/codraw_4.png}}
   \caption{CoDraw manipulation sequence results}
   \label{fig:seq4codraw}
\end{figure}

\begin{figure}[htb!]
  \centering
   \centerline{\includegraphics[width=1\linewidth]{figures/iclevr_2.png}}
   \caption{iCLEVR manipulation sequence results}
   \label{fig:seq2iclevr}
\end{figure}

\begin{figure}[htb!]
  \centering
   \centerline{\includegraphics[width=1\linewidth]{figures/iclevr_3.png}}
   \caption{iCLEVR manipulation sequence results}
   \label{fig:seq3iclevr}
\end{figure}

\begin{figure}[htb!]
  \centering
   \centerline{\includegraphics[width=1\linewidth]{figures/iclevr_4.png}}
   \caption{iCLEVR manipulation sequence results}
   \label{fig:seq4iclevr}
\end{figure}
